# Supplementary material for: Conditional Gaussian Nonlinear System: a Fast Preconditioner and a Cheap Surrogate Model For Complex Nonlinear Systems
Source: arXiv:2112.05226 source file (2021-12-09)
Supplement: Supplementary file 1 [file appendix.tex]

\section{Details of the EM algorithm for parameters estimation}\label{sec: SI_EM}
Consider the discrete fashion of CGNS~\eqref{CGNS} using the Euler-Maruyama scheme~\cite{gardiner2004handbook},
\begin{subequations}\label{eq: discrete forward}
    \begin{align}
    \X^{j+1} = & \X^j + (\A_0(\X^j, t; \btheta) + \A_1(\X^j, t; \btheta) \Y^j) \Delta t + \B_{1}(\X^j, t; \btheta)  \sqrt{\Delta t} \bm{\varepsilon}^j_{1}, \\
    \Y^{j+1} = & \Y^j + (\a_0(\X^j, t; \btheta) + \a_1(\X^j, t; \btheta)\Y^j) \Delta t + \b_{2}(\X^j, t; \btheta) \sqrt{\Delta t} \bm{\varepsilon}^j_{2},
    \end{align}
\end{subequations}
where $\bm{\varepsilon}^j_{1}$ and $\bm{\varepsilon}^j_{2}$ are independent and identically distributed Gaussian white noises that are multidimensional but can have different dimensions from $\X$ and $\Y$, and $\Delta{t}$ is sufficiently small. Assume all the parameters appear as multiplicative prefactors of some functions of $\X^j$ and $\Y^j$ on the right hand side of~\eqref{eq: discrete forward}. Thus, the log likelihood function of $p(\X, \Y | \btheta)$ in M-step can be solved explicitly.

For~\eqref{eq: discrete forward}, the local linear Gaussian approximation on the right hand side is
\begin{equation}
  \cN (\bmu^j, \R^j) = \widetilde{C} |\R^j|^{-\frac{1}{2}} \exp \left(- \frac{1}{2} (\u^{j+1} - \bmu^j)^T (\R^j)^{-1} (\u^{j+1} - \bmu^j)\right),
\end{equation}
where $\u^{j+1} = (\X^{j+1}, \Y^{j+1})^T$ and $\bmu^j = \M^j \bxi  + \S^j$. Here, $\bxi$ is the parameters in the drift part~\eqref{eq: discrete forward} and $\M^j$ is a matrix that includes those linear or nonlinear functions in the drift part which are multiplied by the parameters $\bxi$. On the other hand, $\S^j$ is those terms that do not involve parameters such as the first terms $\X^j$ or $\Y^j$ in~\eqref{eq: discrete forward}. The covariance $\R^j$ is a block diagonal matrix with entries~$(\B_1(\X^j, t))(\B_1(\X^j, t))^* \Delta t$ and~$(\b_2(\X^j, t))(\b_2(\X^j, t))^* \Delta t$, which has a one-to-one correspondence with the parameters in the diffusion terms. The constant $\widetilde{C}$ is due to the normalization of a Gaussian  distribution. Since the states $\Y$ is unobserved and it contains uncertainty, an expectation of the log-likelihood function as in~\eqref{eq: E-step} is adopted, and the overall objective function becomes
\begin{equation}\label{eq: SI_obj}
  \widetilde{\cL} =  \frac{1}{2} \sum_{j}^J \left\langle (\u^{j+1} - \M^j \bxi - \S^j)^* (\R)^{-1} (\u^{j+1} - \M^j \bxi - \S^j) \right\rangle - \frac{J}{2} \log |\R| ,
\end{equation}
where $\bxi$ and $\R$ are parameters in drift terms and diffusion terms, respectively. In~\eqref{eq: SI_obj}, $\left\langle \cdot \right\rangle$ denotes the expectation over the uncertain component of $\u^j$, namely $\Y^j$, at fixed $j$ while the expectation of the observed component $\X^j$ is simply itself. Since the hidden variables $\Y^j$ appears in a linear way, only quadratic terms of $\Y^j$, $\langle \Y^{j + 1}, (\Y^{j + 1})^* \rangle$, $\langle \Y^{j + 1}, (\Y^{j})^* \rangle$, $\langle \Y^{j}, (\Y^{j})^* \rangle$, need to be solved in the expectation in~\eqref{eq: SI_obj}. Details can be found in~\cite{chen2020learning}. Here we assumed $\R^j = \R$ for all $j$.
To find the minimum of~$\widetilde{\cL}$, we aim at finding $\frac{\partial \widetilde{\cL}}{\partial \bxi} =0$ and $\frac{\partial \widetilde{\cL}}{\partial \R} =0$, which leads to
\begin{subequations}\label{eq: SI_Equation_R_Theta}
    \begin{align}
        \R &= \frac{1}{J} \sum_j \left\langle(\u^{j+1} - \M^j \bxi - \S^j)(\u^{j+1} - \M^j\bxi - \S^j)^*\right\rangle, \\
        \bxi &= \D^{-1} \c,
    \end{align}
\end{subequations}
where
\begin{equation}\label{eq: SI_aux_physics_constraint}
	\D = \sum_j \left\langle(\M^j)^*\mathbf{R}^{-1}\M^j\right\rangle \quad \text{and} \quad \c = \sum_j\left\langle(\M^j)^*\mathbf{R}^{-1}(\u^{j+1} - \S^j)\right\rangle.
\end{equation}
Note that we solve~\eqref{eq: SI_Equation_R_Theta} based on an iteration method where~$\bxi$ is obtained given $\R$ from the previous step, and then $\R$ is calculated from the updated $\bxi$.

\subsection{Learning with constraints}\label{sec: EM_constraint}
In certain cases, one may want to constrain the element of $\bxi$. For example, under the restriction
\begin{equation}
	\H \bxi = \g,
\end{equation}
where $\H$ and $\g$ are constant matrices, we obtain the following objective function
\begin{equation}\label{eq: objective_constraint}
	\widetilde{\cL} = \frac{1}{2} \sum_j \left\langle (\u^{j+1} - \M^j \bxi - \S^j)^* (\R)^{-1} (\u^{j+1} - \M^j \bxi - \S^j)\right\rangle - \frac{J}{2}\log |\R^{-1}|  + \blambda^* (\H \bxi - \g).
\end{equation}
Therefore, the solution of the minimization problem with the new objective function~\eqref{eq: objective_constraint} is given as follows
\begin{subequations}\label{eq: SI_Equation_R_Theta_lambda}
    \begin{align}
        \R &= \frac{1}{J} \sum_j \left\langle(\u^{j+1} - \M^j \bxi - \S^j)(\u^{j+1} - \M^j\bxi - \S^j)^*\right\rangle \\
        \blambda &= \left(\H \D^{-1} \H^* \right)^{-1} (\H \D^{-1}\c - \g), \\
        \bxi &= \D^{-1} \left( \c - \H^* \blambda \right),
    \end{align}
\end{subequations}
where $\D$ and $\c$ are defined in~\eqref{eq: SI_aux_physics_constraint}.

\subsection{Learning with block decomposition}\label{sec: EM_block_decomp}

Many complex systems with multiscale structures, multilevel dynamics or state-dependent parameterizations have the following block decomposition features.
Now we develop an efficient strategy with block decomposition and incorporate it into the basic algorithms. Consider the following decomposition of state variables
\begin{equation}
    \u = \bigcup_{i = 1}^I \u_i, \quad \textrm{with} \quad  \u_i = (\X_i, \Y_i),  \quad \X_i \in \bbR^{N_{\I, i}} \quad \textrm{and} \quad \Y_i \in \bbR^{N_{\I\I}, i},
\end{equation}
where $1\le i \le I$, $N_{\I} = \sum_{i = 1}^I N_{\I, i}$ and $N_{\I\I} = \sum_{i = 1}^I N_{\I\I, i}$. Correspondingly, the full dynamics are decomposed into $L$ groups, where the variables on the left-hand side of the $l$th group are $\u_i$. In addition, we assume both $\B_{\mathbf{1}}$ and $\b_{\mathbf{2}}$ are diagonal for notation simplicity. Furthermore, in the dynamics of each $\u_i$ in~\eqref{CGNS}, the terms $\A_{0, i}$ and $\a_{0, i}$ can depend only on the components of $\X_i$ while the terms $\A_{1, i}$ and $\a_{1, i}$ are only functions of $\Y_i$; namely
\begin{equation}
	\begin{aligned}
		\A_{0, i}:=&\A_{0, i}(t, \X), \qquad &\a_{0, i}:=&\a_{0, i}(t, \X), \\
		\A_{1, i}:=&\A_{1, i}(t, \X_i), &\a_{1, i}:=&\a_{1, i}(t, \X_i).
	\end{aligned}
\end{equation}
In addition, only $\Y_i$ involves with terms $\A_{1, i}$ and $\a_{1, i}$. The initial values of $(\X_i, \Y_i)$ and  $(\X_{i'}, \Y_{i'})$ for all $i' \neq i$ are also assumed to be independent with each other. Therefore, we can decompose equation~\eqref{CGNS} as follows,
\begin{subequations}
	\begin{align}
		\frac{\d \X_i (t)}{\d t} =& \left[ \A_{0, i} (\X, t; \bm{\theta}) + \A_{1, i} (\X_i, t; \btheta) \Y_i(t) \right] + \B_{\mathbf{1}}(\X, t; \btheta) \dot{\W}_{\mathbf{1}} (t) ,  \\
		\frac{\d \Y_i (t)}{\d t} =& \left[ \a_{0, i} (\X, t; \btheta) + \a_{1, i} (\X_i, t; \btheta) \Y_i(t) \right] + \b_{\mathbf{2}, i} (\X_i, t; \btheta)  \dot{\W}_{\mathbf{2}, i} (t).
	\end{align}
\end{subequations}
Correspondingly, the evolution of the conditional mean and covariance and smoothing mean and covariance are given as follows
\begin{subequations}\label{eq: filtering block}
	\begin{align}
	\frac{\d \bmu_{\f, i} (t)}{\d t} =& (\a_{0, i} + \a_{0, i} \bmu_{\f, i}) + (\R_{\f, i} \A_{1, i}^*) (\B_{\X, i} \B_{\X, i}^*)^{-1} \left(\frac{\d \X_i}{\d t} - (\A_{0, i} + \A_{1, i} \bmu_{\f, i}) \right),  \\
	\frac{\d \R_{\f, i} (t)}{\d t} =& \left(\a_{1, i} \R_{\f, i} + \R_{\f, i} \a_{1, i}^* + \b_{\mathbf{2}, i} \b_{\mathbf{2}, i}^* - (\R_{\f, i} \A_{1, i}^*) (\B_{\X, i} \B_{\X, i}^*)^{-1} (\A_{1, i} \R_{\f, i})\right),
	\end{align}
\end{subequations}
and

\begin{subequations}\label{eq: smoother block}
	\begin{align}
	  \frac{\overleftarrow{\d \bmu_{\s, i}}}{\d t} &= \big(-\a_{0, i} - \a_{1, i} \bmu_{\s, i}  + ((\b_{\mathbf{2}, i}\b_{\mathbf{2}, i}^*) \R_{\f, i}^{-1} (\bmu_{\f, i} - \bmu_{\s, i}))\big),\\
	  \frac{\overleftarrow{\d \R_{\s, i}}}{\d t} &= -\big((\a_{1, i} + \b_{\mathbf{2}, i}\b_{\mathbf{2}, i}^*) \R_{\f, i}^{-1})\R_{\s, i} + \R_{\s, i} (\a_{1, i}^* + (\b_{\mathbf{2}, i}\b_{\mathbf{2}, i}^*) \R_{\f, i}^{-1}) -(\b_{\mathbf{2}, i}\b_{\mathbf{2}, i}^*) \big.
	\end{align}
\end{subequations}
When computing the log likelihood, we further assumed that the parameters to have a decomposition~$\btheta = \bigcup_{i = 1}^I \btheta_i$, where the parameters~$\btheta_i$ appear only in the equations of $\X_i$ and $\Y_i$. Therefore, the objective function~\eqref{eq: SI_obj} becomes
\begin{equation}
	\begin{aligned}
		\widetilde{\cL} & = \left(\frac{1}{2} \sum_j \left\langle (\u^{j+1} - \M^j \bxi - \S^j)^* (\R)^{-1} (\u^{j+1} - \M^j \bxi - \S^j)\right\rangle - \frac{J}{2} \log |\R^{-1}| \right) \\
		& = \sum_i \left(\sum_j \frac{1}{2} \left\langle (\u_i^{j+1} - \M_i^j \bxi_i - \S_i^j)^* (\R_i)^{-1} (\u_i^{j+1} - \M_i^j \bxi_i - \S_i^j) \right\rangle - \frac{J}{2} \log |\R_i^{-1}| \right).
	\end{aligned}
\end{equation}
Similarly, the optimal solution of the minimization problem of the new objective function of each block can be achieved via
\begin{subequations}\label{eq: Equation_R block}
    \begin{align}
        \mathbf{R}_i &= \frac{1}{J} \sum_j \left\langle(\u_i^{j+1} - \M_i^j \boldsymbol\theta_i - \S_i^j)(\u_i^{j+1} - \M_i^j\bxi_i - \S_i^j)^*\right\rangle, \\
        \bxi_i &= \left(\sum_j \left\langle(\M_i^j)^*\mathbf{R}_i^{-1}\M_i^j\right\rangle\right)^{-1}\left(\sum_j\left\langle(\M_i^j)^*\mathbf{R}_i^{-1}(\u_i^{j+1} - \S_i^j)\right\rangle\right).
    \end{align}
\end{subequations}

\subsubsection{Block decomposition of the approximate two-layer L96 model~\eqref{eq: L96_SP}}\label{sec: EM_L96}
Following general block decomposition from previous section, each block $\u_i$ for the approximate two-layer L96 model~\eqref{eq: L96_SP} is given as $(u_i, v_{l, 1}, v_{l, 2}, \cdots, v_{l, J})$. Correspondingly, $\A_{0, i}$, $\a_{0, i}$, $\A_{1, i}$, $\a_{1, i}$, $\B_{\mathbf{1}, i}$, and $\b_{\mathbf{2}, i}$ are
\begin{equation}
	\begin{aligned}
		\A_{0, i} =& - u_{i - 1} (u_{i - 2} - u_{i + 1}) - u_i + \hat{f}_i,   \qquad \quad
		 \A_{1, i} = (-\hat{a}_i, -\hat{a}_i, \dots, -\hat{a}_i),  \qquad \quad \B_{\mathbf{1}, i}  = \hat{\sigma_u}_i, \\
		\a_{0, i} = & \begin{pmatrix} u_i + \hat{v}_{i, 1} \\
			u_i + \hat{v}_{i, 2} \\
			\vdots \\
			u_i + \hat{v}_{i, J}
		\end{pmatrix},  ~~
		 \a_{1, i} =  \begin{pmatrix} - \hat{d}_{i, 1} & & & \\
			& - \hat{d}_{i, 2} & & \\
			& &  \ddots & \\
			& & & - \hat{d}_{i, J}
		\end{pmatrix},  ~~
		 \b_{\mathbf{2}, i} =  \begin{pmatrix} \hat{\sigma}_{v_{i, 1}} & & & \\
			& \hat{\sigma}_{v_{i, 2}} & & \\
			& &  \ddots & \\
			& & & \hat{\sigma}_{v_{i, J}}
		\end{pmatrix}.
	\end{aligned}
\end{equation}
Therefore, the time evolution of mean and covariance for the filter~\eqref{eq: filtering block} and the smoother~\eqref{eq: smoother block} can be computed in parallel.

\subsection{Higher moments in expectation step}
Recall the general nonlinear system in~\eqref{eq:abs_formu}, it may contain quadratic terms of the hidden variables $\Y$. Therefore, the expectation in~\eqref{eq: SI_obj} might involve up to fourth moments of~$\Y$, which can be calculated by the first two moments utilizing a quasi-Gaussian closure method. For example, denote by $Y_i$ a scalar component of $\Y$. Therefore, the third order moment $\langle Y_i Y_j Y_k \rangle$ and the fourth order moment $\langle Y_i Y_j Y_k Y_m \rangle$ can be obtained as follows
\begin{equation}
  \begin{aligned}
    \langle Y_i Y_j Y_k \rangle &= \mu_i\mu_j\mu_k + \mu_k \sigma_{ij} + \mu_i \sigma_{kj} + \mu_j \sigma_{ik} \\
    \langle Y_i Y_j Y_k Y_m \rangle &= \langle Y_i Y_j Y_k \rangle\mu_m + \mu_i\mu_j \sigma_{km} + \mu_i\mu_k \sigma_{jm} + \mu_k\mu_j \sigma_{im} + \sigma_{ij}\sigma_{km} + \sigma_{ik}\sigma_{jm} + \sigma_{jk}\sigma_{im},
  \end{aligned}
\end{equation}
where $\mu_i$ and $\sigma_{ij}$ are mean and covariance of corresponding components.

\section{Calculating $\cB(\u)$}\label{sec: Bu_form}
In light of~\eqref{eq: FDT_Formula} and~\eqref{Joint_X_Y_Equilibrium_Imperfect}, one has the following explicit expression of $\cB(u)$
\begin{equation}
\begin{aligned}
	\cB(\u) &= - \frac{\textrm{div}_{\u}(\w(\u) \peq^{M | \obs}(\u))}{\peq^{M | \obs}(\u)}\\
&= - \sum_{i = 1}^N \frac{\partial}{\partial{\u_i}}\w_i(\u) - \sum_{i=1}^N \w_i \frac{\partial}{\partial \u_i} \peq^{M | \obs}(\u)\,.
\end{aligned}
\end{equation}
When perturbing the parameters of forcing in the observed processes, the forms of $\cB (\u)$ from the perfect model and the approximate model are the same, since the parameters $F_1$ and $F_2$ appear exactly the same way as in both the perfect and the approximate model. The $\cB(\u)$ term reads as follows
\begin{equation}
	\cB(\u) = - \frac{\partial}{\partial x_1} \peq^{M | \obs}(\u) - \frac{\partial}{\partial x_2} \peq^{M | \obs}(\u)\,.
\end{equation}
When perturbing the parameters in linear interactions terms that appear in both the observed and hidden processes, the formulation of $\cB(\u)$ from the perfect and approximate models are different. Given the perturbation vector $\w(\u) = (y_1, y_2, -x_1, -x_2)^{\top}$, the $\cB(\u)$ from the perfect model is as follows
\begin{equation}
	\cB(\u) = - y_1 \frac{\partial}{\partial x_1} \peq^{M | \obs}(\u) - y_2 \frac{\partial}{\partial x_2} \peq^{M | \obs}(\u) + x_1 \frac{\partial}{\partial y_1} \peq^{M | \obs}(\u) + x_2 \frac{\partial}{\partial y_2} \peq^{M | \obs}(\u)\,.
\end{equation}
However, since there is no $L_{13}$ and $L_{24}$ parameters in the hidden processes of the approximate model, the formulation of $\cB(\u)$ from the approximate model remains
\begin{equation}
	\cB(\u) = - y_1 \frac{\partial}{\partial x_1} \peq^{M | \obs}(\u) - y_2 \frac{\partial}{\partial x_2} \peq^{M | \obs}(\u).
\end{equation}
